# Supplementary material for: Learning to Coordinate for a Worker-Station Multi-robot System in Planar Coverage Tasks
Source: arXiv:2208.02993 source file (2022-08-24)
Supplement: Supplementary file 1 [file p_appendix.tex]

\section*{APPENDIX}
